# Supplementary material for: Cost-Aware Best-LLM Identification using Dueling Feedback
Source: arXiv:2609.30360 source file (2026-09-24)
Supplement: Supplementary file 1 [file proofs_old.tex]

\section{Missing Proofs of Lemmas and Theorems}
\label{app: missing proofs}

In this section, we provide complete proofs of the results stated in the main text. We begin in Appendix~\ref{app: lower bound} with the derivation of the lower bound.

%%%%%%%%%%%%%%%%%%%%%%%%%%%%%%%%%%%%%%%%%%%%%%%%%%%%%%%%%%%%%%%%%%%%%%%%%%%

\subsection{Lower Bound}
\label{app: lower bound}

\begin{proof}[Proof of Lemma \ref{lemma:lower_bound_abstract}:]
The result is straightforward when \( E_{\nu}[J(\tau_{\delta})] = \infty \). Hence, for the rest of the proof, we assume that \( E_{\nu}[J(\tau_{\delta})] < \infty \implies E_{\nu}[N(\tau_{\delta})] < \infty \), where \( E_{\nu}[N(\tau_{\delta})] \) is the expected number of total pulls made by any \( \delta \)-PC algorithm. Consequently, we have \( P_{\nu}(\tau_\delta = \infty) = 0 \).

Next, let $\nu' \in \epsilon_{\text{alt}} \left(\nu\right)$, and let $E$ be the event defined as $E = \{\tau_{\delta} < \infty \text{ and } o \notin a^*\left(\nu'\right)\}$, where $o \in \mathcal{L}$ is the output arm recommended at the stopping time. Then, we have 
\begin{align}
    2\delta &\geq  P_{\nu}\left(\tau_\delta < \infty \text{ and } o \notin a^*\left(\nu\right)\right) +  P_{\nu'}\left(\tau_\delta < \infty \text{ and } o \notin a^*\left(\nu'\right)\right) \label{lb1eq1}\\
    &\geq P_{\nu}\left(E^c\right) + P_{\nu'}\left(E\right) \label{lb1eq2}\\
    &\geq \dfrac{1}{2} \exp{\left( -\sum_{(i,j)\in\mathcal{K}} E_{\nu}[N_{i,j}\left(\tau_{\delta}\right)] d\left(p_{i,j}, p'_{i,j}\right) \right)} \label{lb1eq3}
\end{align}
Rearranging \eqref{lb1eq3} gives
\begin{align}
    \log\left(\dfrac{1}{4\delta} \right) \leq \sum_{(i,j)\in\mathcal{K}} E_{\nu}[N_{i,j}\left(\tau_{\delta}\right)] d\left(p_{i,j}, p'_{i,j}\right) \label{lb2eq1}
\end{align}
Now, we choose an instance $\nu' \in \epsilon_{\text{alt}}\left(\nu\right)$ that gives a different answer than $\nu$ to achieve the infimum on the right hand side of \eqref{lb2eq1}, giving 
\begin{align}
    \log\left(\dfrac{1}{4\delta} \right) &\leq \inf_{\bm{\nu}' \in \epsilon_{\text{alt}}\left(\nu\right)} \left( \sum_{(i,j)\in\mathcal{K}} E_{\nu}[N_{i,j}\left(\tau_{\delta}\right)] d\left(p_{i,j}, p'_{i,j}\right) \right) \label{lb3eq1} \\
    &= E_{\nu}[J\left(\tau_\delta\right)] \left( \inf_{\bm{\nu}' \in \epsilon_{\text{alt}}\left(\nu\right)} \left( \sum_{(i,j)\in\mathcal{K}} \dfrac{E_{\nu}[N_{i,j}\left(\tau_{\delta}\right)]}{E_{\nu}[J\left(\tau_\delta\right)]} d\left(p_{i,j}, p'_{i,j}\right) \right) \right) \label{lb3eq2} \\
    &= E_{\nu}[J\left(\tau_\delta\right)] \left( \inf_{\bm{\nu}' \in \epsilon_{\text{alt}}\left(\nu\right)} \left( \sum_{(i,j)\in\mathcal{K}} \dfrac{E_{\nu}[N_{i,j}\left(\tau_{\delta}\right)]}{\sum_{(m,n)\in\mathcal{K}} \left(c_m+c_n\right) E_{\nu}[N_{i,j}\left(\tau_\delta\right)]} d\left(p_{i,j}, p'_{i,j}\right)  \right) \right)\label{lb3eq3} \\
    &= E_{\nu}[J\left(\tau_\delta\right)] \left( \inf_{\bm{\nu}' \in \epsilon_{\text{alt}}\left(\nu\right)} \left( \sum_{(i,j)\in\mathcal{K}} \dfrac{1}{\left(c_i+c_j\right)} \dfrac{\left(c_i+c_j\right)E_{\nu}[N_{i,j}\left(\tau_{\delta}\right)]}{\sum_{(m,n)\in\mathcal{K}} \left(c_m+c_n\right) E_{\nu}[N_{i,j}\left(\tau_\delta\right)]} d\left(p_{i,j}, p'_{i,j}\right) \right) \right) \label{lb3eq4} 
\end{align}
Now, we let $w_{i,j} = \frac{\left(c_i+c_j\right)E_{\nu}[N_{i,j}\left(\tau_{\delta}\right)]}{\sum_{(m,n)\in\mathcal{K}} \left(c_m+c_n\right) E_{\nu}[N\left(\tau_\delta\right)]}$ be the proportion of cost incurred by pulling the arm pair $i$ and $j$. Note that the summation across all $w_{i,j}$ pairs is equal to $1$, giving us
\begin{align}
    \log\left(\dfrac{1}{4\delta} \right) &\leq E_{\nu}[J\left(\tau_\delta\right)] \left( \inf_{\bm{\nu}' \in \epsilon_{\text{alt}}\left(\nu\right)} \left( \sum_{(i,j)\in\mathcal{K}} \dfrac{w_{i,j}}{\left(c_i+c_j\right)} d\left(p_{i,j}, p'_{i,j}\right)\right) \right) \label{lb4eq1}
\end{align}
Then, we can further upper bound the above expression by taking the supremum over $\mathbf{w}$, giving
\begin{align}
    \log\left(\dfrac{1}{4\delta} \right) \leq E_{\nu}[J\left(\tau_\delta\right)] \left(\sup_{\mathbf{w} \in \sum_{K}} \left( \inf_{\bm{\nu}' \in \epsilon_{\text{alt}}\left(\nu\right)} \left( \sum_{(i,j)\in\mathcal{K}} \dfrac{w_{i,j}}{\left(c_i+c_j\right)} d\left(p_{i,j}, p'_{i,j}\right) \right) \right) \right) \leq E_{\nu}[J\left(\tau_\delta\right)] c^*\left(\nu\right)^{-1} \label{lb5eq1}
\end{align}
Therefore, we have a lower bound on the total cost given by 
\begin{align}
     E_{\nu}[J\left(\tau_\delta\right)] \geq c^*\left(\nu\right) \log\left(\dfrac{1}{4\delta} \right) \label{lb6eq1}
\end{align}
Hence, completing the proof
\end{proof}

\begin{proof}[Proof of Theorem \ref{theorem: minmax}]
Without loss of generality, let us assume the Condorcet winner to be arm $1$. The bound in Theorem \ref{theorem: minmax} is attained by optimally allocating the weights $w_{i,j}$ across the set of arms. More formally, to obtain an interpretable lower bound, we compute the optimal cost proportion of these weights by solving the following optimization problem, which is motivated by Lemma \ref{lemma:lower_bound_abstract}. We begin by simplifying Equation \ref{eq:lower_bound_generic} into the following discrete minimization form:
\begin{align}
    c^*\left(\nu\right)^{-1} &= \sup_{\mathbf{w} \in \Sigma_{\K}} \ \inf_{\nu' = (\mathcal{C},\mathbb{P}') \in \epsilon_{\text{alt}} \left(\nu\right)}\ 
    \left( \sum_{(i,j) \in \K} \dfrac{w_{i,j}}{c_i + c_j} d\left(p_{i,j}, p'_{i,j} \right) \right) \label{eq1}\\
    &= \sup_{\mathbf{w} \in \sum_{K}}  \min_{i \neq 1} \left( \sum_{j \neq i } \dfrac{w_{i,j}}{c_i + c_j} d\left(p_{i,j}, \max{(0.5, p_{i,j})}\right) \right) \label{eq2}
\end{align}
where the second line reformulates the inner infimum as a discrete minimization over suboptimal arms. 

Accordingly, the optimal weight allocation is given by:
\begin{align}
    w\left( \nu \right) &= \argmax_{\mathbf{w} \in \sum_{K}} \left( \min_{i \neq 1} \left( \sum_{j \in \mathcal{L} \backslash i } \dfrac{w_{i,j}}{c_i + c_j} d\left(p_{i,j}, \max{(0.5, p_{i,j})}\right) \right) \right) \label{mssr2eq1}
\end{align}
It is easy to see that, at the optimum, the quantities inside the minima i.e $\sum_{j \in \mathcal{L} \backslash i } \frac{w_{i,j}}{c_i + c_j} d\left(p_{i,j}, \max{(0.5, p_{i,j})}\right)$ are all equal.
Thus, $w$ can be calculated by simply solving the $L$ linear equations, out of which $L-1$ belong to the inner minima of the equation \eqref{mssr2eq1} and the remaining equation comes from the constraint on the weight vector. However, note that the optimal weights may not be unique for the instances when there exists an $i \neq 1$, such that there exists $j_1, j_2$ satisfying
\begin{align}
   \dfrac{ d\left(p_{i,j_1}, 0.5\right)}{c_i + c_{j_1}} = \dfrac{ d\left(p_{i,j_2}, 0.5\right)}{c_i + c_{j_2}} = \max_{j \neq i}\dfrac{ d\left(p_{i,j}, 0.5\right)}{c_i + c_{j}} \label{mssr3eq1}
\end{align}
Now let us define $\mathcal{W}^*\left(\nu\right)$ to be the set of weight vectors that attain supremum in \eqref{mssr2eq1} and $w_i$ to be the sum of weights involving $w_{i,.}$. Formally $w_i = \sum_{j \in \mathcal{L} \backslash i} w_{i,j}$. We then have 
\begin{align}
    w_i &= 1 \Bigg/ \sum_{m \in L} \dfrac{\max_{j \neq i}\left(\dfrac{1}{c_i + c_j} d\left(p_{i,j}, \max{(0.5, p_{i,j})}\right)\right)}{\left(\max_{n \neq m}\left(\dfrac{1}{c_m + c_n} d\left(p_{m,n}, \max{(0.5, p_{m,n})}\right)\right)\right)}
    \label{mssr4eq1}
\end{align}
Next, for every $i$ not satisfying \eqref{mssr3eq1}, it is easy to see that
\begin{align*}
w_{i,j} =
\begin{cases}
0, & \text{if }\begin{aligned}[t]
&\displaystyle \max_{k\neq i}\!\left(\frac{1}{c_i+c_k}\,
  d\Bigl(p_{i,k},\, \max\{0.5,\, p_{i,k}\}\Bigr)\right) \\
&\displaystyle > \frac{1}{c_i+c_j}\,
  d\Bigl(p_{i,j},\, \max\{0.5,\, p_{i,j}\}\Bigr)
\end{aligned} \\
w_i, & \text{otherwise.}
\end{cases}
\end{align*}
On the other hand, for all values of $i$ satisfying \eqref{mssr3eq1}, the weight $w_i$ can be distributed as any linear combination of weights corresponding to all $j$ satisfying \eqref{mssr3eq1}. Finally, on substituting one of the weight vectors $\mathcal{W}^*\left(\nu\right)$ in Equation \ref{eq2}, we get our desired result.
\end{proof}

%%%%%%%%%%%%%%%%%%%%%%%%%%%%%%%%%%%%%%%%%%%%%%%%%%%%%%%%%%%%%%%%%%%%%%%%%%%%

\subsection{Closed form solution for GLR statistic}

\begin{proof}[Proof of Lemma \ref{lemma: mssr1eq1}:]
    We start by identifying the unrestricted likelihood estimate ($L\left(p\right)$) of the log-likelihood function
\begin{align}
    L\left(p\right) &= \left(N^1_{i,j}\left(t\right)\right) \log\left(p_{i,j}\right) + \left(N-N^1_{i,j}\left(t\right)\right)\log\left(1-p_{i,j}\right) \label{sr11eq1} \\
    &= N_{i,j}\left(t\right) [\hat{p}_{i,j}\left(t\right)\log\left(p_{i,j}\right) + \left(1-\hat{p}_{i,j}\left(t\right)\right)\log\left(1-p_{i,j}\right) \label{sr11eq2}]
\end{align}
On differentiation \eqref{sr11eq2} and equating to $0$, we obtain $p_{i,j} = \hat{p}_{i,j}\left(t\right)$. However, since we have constraints on $p_{i,j}$ with $0.5$ being the boundary value, we have 
\begin{equation}
\label{sr12eq1}
p_{i,j} =
\begin{cases}
  \min\left(\hat{p}_{i,j}\left(t\right), 0.5\right), & \text{if}\ p_{i,j} < 0.5\\
  \max\left(\hat{p}_{i,j}\left(t\right), 0.5\right), & \text{otherwise}
\end{cases}
\end{equation}
Furthermore, it follows that
\begin{align}
    Z_{i,j}\left(t\right) &= \log \dfrac{\max_{\text{i is best}} \prod_{m=1}^{L-1} \prod_{n=m+1}^L \left(p_{m,n}\right)^{N_{m,n}\left(t\right) \hat{p}_{m,n}\left(t\right)} \left(1-p_{m,n}\left(t\right)\right)^{N_{m,n}\left(t\right) \left(1 - \hat{p}_{m,n}\left(t\right) \right)}}{\max_{\text{j is best}} \prod_{m=1}^{L-1} \prod_{n=m+1}^L \left(p_{m,n}\right)^{N_{m,n}\left(t\right) \hat{p}_{m,n}\left(t\right)} \left(1-p_{m,n}\left(t\right)\right)^{N_{m,n}\left(t\right) \left(1 - \hat{p}_{m,n}\left(t\right) \right)}} \label{sr14eq1} \\
    &= \resizebox{\columnwidth}{!}{$
    \log \dfrac{\prod_{k \in \mathcal{L}} \left(\max\left(\hat{p}_{i,k}\left(t\right), 0.5 \right)\right)^{N_{i,k}\left(t\right) \hat{p}_{i,k}\left(t\right)} \left(1-\max\left(\hat{p}_{i,k}\left(t\right), 0.5 \right)\right)^{N_{i,k}\left(t\right)\left(1- \hat{p}_{i,k}\left(t\right)\right)} \prod_{k \in \mathcal{L} \backslash i} \left(\hat{p}_{j,k}\left(t\right)\right)^{N_{j,k}\left(t\right) \hat{p}_{j,k}\left(t\right)} \left(1-\hat{p}_{j,k}\left(t\right)\right)^{N_{j,k}\left(t\right)\left(1- \hat{p}_{j,k}\left(t\right)\right)}}{\prod_{k \in \mathcal{L}} \left(\max\left(\hat{p}_{j,k}\left(t\right), 0.5 \right)\right)^{N_{j,k}\left(t\right) \hat{p}_{j,k}\left(t\right)} \left(1-\max\left(\hat{p}_{j,k}\left(t\right), 0.5 \right)\right)^{N_{j,k}\left(t\right)\left(1- \hat{p}_{j,k}\left(t\right)\right)} \prod_{k \in \mathcal{L} \backslash j} \left(\hat{p}_{i,k}\left(t\right)\right)^{N_{i,k}\left(t\right) \hat{p}_{i,k}\left(t\right)} \left(1-\hat{p}_{i,k}\left(t\right)\right)^{N_{i,k}\left(t\right)\left(1- \hat{p}_{i,k}\left(t\right)\right)} }$} \label{sr14eq2} \\
    &= \resizebox{\columnwidth}{!}{$
    \sum_{k \in \mathcal{L}} N_{j,k}\left(t \right) \log \left( \dfrac{(\hat{p}_{j,k}\left(t \right))^{\hat{p}_{j,k}\left(t\right)} (1-\hat{p}_{j,k}\left(t \right))^{(1 - \hat{p}_{j,k}\left(t\right)}}{\left(\max\left(\hat{p}_{j,k}\left(t\right), 0.5\right)\right)^{\hat{p}_{j,k}\left(t\right)} \left(1-\max\left(\hat{p}_{j,k}\left(t\right), 0.5\right)\right)^{(1 - \hat{p}_{j,k}\left(t\right)}} \right) - \sum_{k \in \mathcal{L}} N_{i,k}\left(t\right) \log \left( \dfrac{(\hat{p}_{i,k}\left(t\right))^{\hat{p}_{i,k}\left(t\right)} (1-\hat{p}_{i,k}\left(t\right))^{(1 - \hat{p}_{i,k}\left(t\right)}}{\left(\max\left(\hat{p}_{i,k}\left(t\right), 0.5\right)\right)^{\hat{p}_{i,k}\left(t\right)} \left(1-\max\left(\hat{p}_{i,k}\left(t\right), 0.5\right)\right)^{(1 - \hat{p}_{i,k}\left(t\right)}} \right)$} \label{sr14eq3} \\ 
    &= \sum_{k \in \mathcal{L}} N_{j,k}\left(t\right) d(\hat{p}_{j,k}\left(t\right), \max(\hat{p}_{j,k}\left(t\right), 0.5)) - \sum_{k \in \mathcal{L}} N_{i,k}\left(t\right) d\left(\hat{p}_{i,k}, \max\left(\hat{p}_{i,k}\left(t\right), 0.5\right)\right) \label{sr14eq4}
\end{align}
\end{proof}

\subsection{Correctness Argument}

\begin{definition}
\label{def: rank}
    Consider a sequential identification problem specified by a partition \( \mathcal{O} = \bigcup_{i=1}^{L} \mathcal{O}_i \), where each \( \mathcal{O}_i \) represents a open set where arm \( i \) is the correct answer. Then the rank $R$ of the problem is defined as the minimum number of arms required to describe the exclusion of any set \( \mathcal{O}_i \) from the set \( \mathcal{O} \). More specifically, the set \( \mathcal{O} \setminus \mathcal{O}_i \) can be expressed as a finite union of conditions involving at most \( R \) arms.
\end{definition}

\begin{lemma}
\label{lemma: delta}
 For any sequential identification problem, let $R$ be its rank, and $M$ be the number of open sets. Then, from Preposition 21 of \cite{kaufmann2021mixture} we know that the Generalized Likelihood Ratio Test (GLRT) stopping rule is \( \delta \)-correct with threshold
    \begin{align}
        \gamma\left(t, \delta \right) = 3R\log\left(1 + \log\left(\frac{t}{R}\right)\right) + R C\left(\dfrac{\log\left(\frac{M-1}{\delta} \right)}{R} \right) \label{delta}
    \end{align}
\end{lemma}

\begin{proof}[Proof of Theorem \ref{theorem: delta-pac}:]
    We know that the probability that the algorithm stops and outputs the wrong answer is bounded by
\begin{align}
     P_{\nu}\left(\tau_\delta < \infty, \hat{a}_{\tau_\delta} \neq a^*\left(\nu\right)\right) &\leq P_{\nu}\left(\exists b \in \mathcal{L} \backslash a^*\left(\nu\right), \exists t \in \mathbb{N} \mid \forall i \in \mathcal{L} \backslash b \; Z_{b, i}\left(t\right) > \beta\left(t, \delta\right)\right) \label{pc1eq1}\\
     &\leq P_{\nu}\left(\exists b \in \mathcal{L} \backslash a^*\left(\nu\right), \exists t \in \mathbb{N} \mid  Z_{b, a^*\left(\nu\right)}\left(t\right) > \beta\left(t, \delta\right)\right) \label{pc1eq2}
\end{align}
For the above event, we have
\begin{align}
    Z_{b, a^*\left(\nu\right)} \left(t\right) &= \sum_{k \in \mathcal{L}} N_{a^*\left(\nu\right),k}\left(t\right) d(\hat{p}_{a^*\left(\nu\right),k}\left(t\right), \max(\hat{p}_{a^*\left(\nu\right),k}\left(t\right), 0.5)) - \sum_{k \in \mathcal{L}} N_{b,k}\left(t\right) d\left(\hat{p}_{b,k}, \max\left(\hat{p}_{b,k}\left(t\right), 0.5\right)\right) \label{pc2eq1}\\
    &\leq \sum_{k \in \mathcal{L}} N_{a^*\left(\nu\right),k}\left(t\right) d\left(\hat{p}_{a^*\left(\nu\right),k}\left(t\right), \max\left(\hat{p}_{a^*\left(\nu\right),k}\left(t\right), 0.5\right)\right) \label{pc2eq2}
\end{align}
Furthermore, we also have 
\begin{equation}
\label{pc3eq1}
N_{a^*\left(\nu\right),k}\left(t\right) d\left(\hat{p}_{a^*\left(\nu\right),k}\left(t\right), \max\left(\hat{p}_{a^*\left(\nu\right),k}\left(t\right), 0.5\right)\right) =
\begin{cases}
   N_{a^*\left(\nu\right),k}\left(t\right) d\left(\hat{p}_{a^*\left(\nu\right),k}\left(t\right), 0.5\right) & \text{if}\ \hat{p}_{a^*\left(\nu\right),k}\left(t\right) < 0.5\\
   0 & \text{otherwise}
\end{cases}
\end{equation}
Therefore, we can write
\begin{align}
     Z_{b, a^*\left(\nu\right)} \left(t\right) &\leq \sum_{k \in \mathcal{L}} N_{a^*\left(\nu\right),k}\left(t\right) d\left(\hat{p}_{a^*\left(\nu\right),k}\left(t\right),  p_{a^*\left(\nu\right),k}\right) \label{pc4eq1}
\end{align}
Now, we bound the error probability as follows 
\begin{align}
    P_{\nu}\left(\tau_\delta < \infty, \hat{a}_{\tau_\delta} \neq a^*\left(\nu\right)\right) &\leq P_{\nu}\left(\exists b \in \mathcal{L} \backslash a^*\left(\nu\right), \exists t \in \mathbb{N} \mid \sum_{k \in \mathcal{L}} N_{a^*\left(\nu\right),k}\left(t\right) d\left(\hat{p}_{a^*\left(\nu\right),k}\left(t\right),  p_{a^*\left(\nu\right),k}\right) > \beta\left(t, \delta\right)\right) \label{pc5eq1}
\end{align}
From the definition of rank (refer to Definition \ref{def: rank}), we see that for our problem, we have rank $R = L-1$ and the number of open sets $M = L$. Finally, on substituting the values of $R$ and $M$ in \eqref{delta}, the expression of $\gamma\left(t, \delta\right)$ is exactly equivalent to $\beta\left(t, \delta\right)$, hence giving us
\begin{align}
    P_{\nu}\left(\tau_\delta < \infty, \hat{a}_{\tau_\delta} \neq a^*\left(\nu\right)\right) &\leq \delta \label{pc6eq1}
\end{align}
\end{proof}

\subsection{Cost Complexity}

\begin{lemma}
\label{lemma: hemicontinous}
    The mapping $\nu \mapsto \alpha^*\left(\nu\right)$ is upper hemicontinuous and compact-valued. Furthermore, the set $\alpha^*\left(\nu\right)$ is convex for every instance $\nu \in \epsilon$
\end{lemma}

\textbf{Proof of Lemma \ref{lemma: hemicontinous}:}
To establish the upper hemicontinuity and compactness of the mapping $\nu \mapsto \alpha^*\left( \nu \right)$, we begin by proving the compactness of set $\mathcal{W}^*\left(\nu\right)$. Recall that $\mathcal{W}^*\left(\nu\right)$ is defined by
\begin{align}
    \mathcal{W}^*\left( \nu \right) &= \argmax_{\bf{w} \in \sum_{\mathcal{K}}}\left\{\min_{i \neq 1} \left( \sum_{j \in \mathcal{L} \backslash i } \dfrac{w_{i,j}}{c_i + c_j} d\left(p_{i,j}, \max{(0.5, p_{i,j})}\right) \right)\right\} \label{hc1eq1}
\end{align}
Further, we also know that $\sum_K$ is a $K$-dimensional simplex, meaning it's closed and bounded and hence a compact set. Since the feasible set $\sum_K$ is compact and $\mathcal{W}^*\left( \nu \right)$ is continuous, any set of maximizers $\mathcal{W}^*\left( \nu \right) \subseteq \sum_K$ will also be a compact set. Now, given that there's a bijective mapping from set $\mathcal{W}^* \left(\nu\right)$ to $\alpha^*\left(\nu\right)$ and the function $f\left(\mathcal{W}^*, C\right)$ and it's inverse are continuous, we also have $\alpha^*\left(\nu\right)$ to be compact as well.

Next, let $\phi\left(\nu, \alpha\right)$ be defined as
\begin{align}
    \phi\left(\nu, \alpha\right) &= \min_{i \neq 1} \left( \sum_{j \in \mathcal{L} \backslash i } \dfrac{\alpha_{i,j}}{\sum_{(m,n) \in \mathcal{K}} \alpha_{m,n} (c_m + c_n)} d\left(p_{i,j}, \max{(0.5, p_{i,j})}\right) \right)  \label{hc2eq1} \\
    &= \dfrac{1}{\sum_{(m,n) \in \mathcal{K}} \alpha_{m,n} (c_m+c_n)} \min_{i \neq 1} \left(\sum_{j \in \mathcal{L} \backslash i} \alpha_{i,j}d\left(p_{i,j}, \max{(0.5, p_{i,j})}\right) \right)  \label{hc2eq2}
\end{align}
From \eqref{hc2eq2}, we see that $\phi\left(\nu, \alpha\right)$ is a function of two continuous functions and hence is continuous as well. Now, from the definition of $\mathcal{W}^*\left(\nu\right)$ and the mapping function $f\left( \mathcal{W}^*, \mathcal{C}\right)$, we know that $\alpha^*\left(\nu\right)$, can also be written as 
\begin{align}
    \alpha^*\left(\nu\right) &= \argmax_{\bf{\alpha}\in\sum_{\mathcal{K}}}\left\{\min_{i \neq 1} \left( \sum_{j \in \mathcal{L} \backslash i } \dfrac{\alpha_{i,j}}{\sum_{(m,n) \in \mathcal{K}} \alpha_{m,n}(c_m + c_n)} d\left(p_{i,j}, \max{(0.5, p_{i,j})}\right) \right)\right\} \label{hc3eq1}
\end{align}
Therefore, given that $\sum_{\mathcal{K}}$ is compact valued, meaning for every instance $\nu \in \epsilon$, there exists a set of feasible weight allocations, and the objective function $\phi\left(\nu, \alpha\right)$ is continuous in $\nu$ and $\alpha$, from the Berge maximum theorem, we say that the set of maximizers i.e $\alpha^*\left(\nu\right)$ is upper hemicontinuous with nonempty and compact values.

We now show that $\alpha^*\left(\nu\right)$ is convex for all $\nu$. Let us fix the instance $\nu$, and pick $\alpha^{\left(1\right)}, \alpha^{\left(2\right)} \in \alpha^*\left(\nu\right)$ and arbitrarily choose $z \in \left[0,1\right]$. From the definition, we have 
\begin{align}
    \phi\left(\nu, \alpha^{\left(1\right)}\right) = \phi\left(\nu, \alpha^{\left(2\right)}\right) = c^*\left(\nu\right)^{-1} \label{hc4eq1}
\end{align}
We then have
\begin{align}
    \phi\left(\nu, z\alpha^{\left(1\right)} + \left(1-z\right)\alpha^{\left(2\right)}\right) &= \min_{i\neq1}\left(\sum_{j\in \mathcal{L} \backslash i}\dfrac{z\alpha_{i,j}^{\left(1\right)} + \left(1-z\right)\alpha^{\left(2\right)}_{i,j}}{\sum_{(m,n)\in\mathcal{K}} \left(z\alpha_{m,n}^{\left(1\right)} + \left(1-z\right)\alpha^{\left(2\right)}_{m,n}\right) (c_m + c_n)} d\left(p_{i,j}, \max{(0.5, p_{i,j})}\right)\right) \label{hc5eq1} \\
    &\geq z\min_{i\neq1}\left(\sum_{j\in \mathcal{L} \backslash i}\dfrac{\alpha_{i,j}^{\left(1\right)}}{\sum_{(m,n)\in\mathcal{K}} \left(z\alpha_{m,n}^{\left(1\right)} + \left(1-z\right)\alpha^{\left(2\right)}_{m,n}\right) (c_m+c_n)} d\left(p_{i,j}, \max{(0.5, p_{i,j})}\right)\right) \nonumber \\ &+ \left(1-z\right)\min_{i\neq1}\left(\sum_{j\in \mathcal{L} \backslash i}\dfrac{\alpha^{\left(2\right)}_{i,j}}{\sum_{(m,n)\in\mathcal{K}} \left(z\alpha_{m,n}^{\left(1\right)} + \left(1-z\right)\alpha^{\left(2\right)}_{m,n}\right) (c_m + c_n)} d\left(p_{i,j}, \max{(0.5, p_{i,j})}\right) \right) \label{hc5eq2} \\
    &= z\min_{i\neq1}\left(\sum_{j\in \mathcal{L} \backslash i}\dfrac{w_{i,j}^{\left(1\right)}/\left(c_i+c_j\right)}{\sum_{(m,n)\in\mathcal{K}} \left(zw_{m,n}^{\left(1\right)}/(c_m + c_n) + \left(1-z\right)w^{\left(2\right)}_{m,n}/(c_m+c_n)\right) (c_m + c_n)} d\left(p_{i,j}, \max{(0.5, p_{i,j})}\right)\right) \nonumber \\ &+ \left(1-z\right)\min_{i\neq1}\left(\sum_{j\in \mathcal{L} \backslash i}\dfrac{w_{i,j}^{\left(2\right)}/\left(c_i+c_j\right)}{\sum_{(m,n)\in\mathcal{K}} \left(zw_{m,n}^{\left(1\right)}/(c_m + c_n) + \left(1-z\right)w^{\left(2\right)}_{m,n}/(c_m + c_n)\right) (c_m+c_n)} d\left(p_{i,j}, \max{(0.5, p_{i,j})}\right)\right) \label{hc5eq3} \\
    &= z \min_{i\neq 1} \left( \sum_{j\in \mathcal{L}\backslash i}\dfrac{w^{\left(1\right)}_{i,j}}{c_i + c_j} d\left(p_{i,j}, \max{(0.5, p_{i,j})}\right) \right) + \left(1-z\right) \min_{i \neq 1} \left(\sum_{j\in \mathcal{L} \backslash i}\dfrac{w^{\left(2\right)}_{i,j}}{c_i + c_j} d\left(p_{i,j}, \max{(0.5, p_{i,j})}\right)\right) \label{hc5eq4} \\
    &= z c^*\left(\nu\right)^{-1} + \left(1-z\right) c^*\left(\nu\right)^{-1} \label{hc5eq5} \\
    &= c^*\left(\nu\right)^{-1} \label{hc5eq6}
\end{align}
Also as $\sum_K$ is convex, $z\alpha^{\left(1\right)} + \left(1-z\right) \alpha^{\left(2\right)} \in \sum_K$ indicating $\phi\left(\nu, z\alpha^{\left(1\right)} + \left(1-z\right) \alpha^{\left(2\right)} \right)\leq c^*\left(\nu\right)^{-1}$ thus implying that $\phi\left(\nu, z\alpha^{\left(1\right)} + \left(1-z\right)\alpha ^{\left(2\right)} \right) = c^*\left(\nu\right)^{-1}$. This proves that $z \alpha^{\left(1\right)} + \left(1-z\right) \alpha^{\left(2\right)} \in \alpha^*\left(\nu\right)$ and thus the set $\alpha^*\left(\nu\right)$ is convex in nature. 

Next, given real-valued vectors $u, v$ of identical sizes and a compact, convex set $S$, we define $d_\infty\left(u,v\right) := \max_i|u_i-v_i|$, $d_\infty\left( u, S\right):= \min_{v \in S} d_\infty\left(u,v\right)$, and $||u-v|| := \sqrt{\sum_i\left( u_i - v_i\right)^2}$


\begin{lemma}
\label{lemma: tracking}
    Under the tracking rule given in lines 3 to 7 of Algorithm \ref{algo: DCTAS}, we have almost surely
    \begin{align}
    \label{l2eq1}
    \lim_{t \rightarrow \infty} d_\infty \left(\left( N_{i,j}\left(t\right)/t\right)_{i,j \in \mathcal{L}}, \alpha^*\left(\nu\right)\right) = 0 
    \end{align}
\end{lemma}

\textbf{Proof of Lemma \ref{lemma: tracking}:}
Let $S:=\alpha^*\left(\nu\right)$. Next for a fix $\epsilon > 0$, from the sampling rule we have $N_{i,j}\left(t\right) = \Omega\left(\sqrt{t}\right)$ almost surely for $i,j \in \mathcal{L}$. This implies by the strong law of large numbers that $||\hat{\nu}\left(t\right) - \nu|| \xrightarrow{t \rightarrow \infty} 0$ almost surely. Also as $\alpha\left(t+1\right) \in \alpha^*\left(\hat{\nu}\right)$ for all $t$ and $\alpha^*\left(\hat{\nu}\right)$ is close to $S$ for large $t$, from the upper hemicontinuity of mapping (refer Lemma \ref{lemma: hemicontinous}), we know that there exists $t_0 = t_0\left(\epsilon\right)$ such that for all $t \geq t_0$ we have $d_\infty\left( \alpha\left(t\right), S\right) \leq \epsilon$. Now, if $v\left(t\right) := \argmin_{\alpha \in S} d_\infty\left(\alpha\left(t\right), \alpha \right)$ denote the projection of $\alpha\left(t\right)$ onto $S$, then we have $d_\infty\left(\alpha\left(t\right), v\left(t\right)\right) \leq \epsilon$ for all $t \geq t_0$. Letting  $\bar{v}\left(t\right) := \frac{1}{t} \sum_{s=1}^t v\left(s\right)$ and  $\bar{\alpha}\left(t\right) := \frac{1}{t} \sum_{s=1}^t \alpha\left(s\right)$, we have $||\bar{\alpha}\left(t\right) - \bar{v}\left(t\right)|| \leq 9\epsilon, \; \forall t > t_0' = t_0/8\epsilon$ (refer \cite{reddy2023best}). On letting $\hat{\alpha}\left(t\right) := \argmin_{\alpha \in S} d_\infty\left(\bar{\alpha}\left(t\right), \alpha\right)$, we have $d_\infty\left( \bar{\alpha}\left(t\right), \hat{\alpha}\left(t\right)\right) \leq 9\epsilon$ for all $t \geq t_0'$ \\
Next, we define $\epsilon_{i,j} \left(t\right) := N_{i,j}\left(t\right) - t \bar{\alpha}_{i,j} \left(t\right), \; \forall i,j \in \mathcal{L}, t$. Therefore, we have
\begin{align}
    \epsilon_{i,j}\left(t+1\right) &= N_{i,j}\left(t+1\right) - \left(t+1\right) \bar{\alpha}_{i,j} \left(t+1\right) \label{le1eq1} \\
    &= N_{i,j}\left(t\right) + \mathbb{1}\left(a_{t+1} = i,j \right) - \left(t+1\right) \bar{\alpha}_{i,j} \left(t+1\right) \label{le1eq2} \\
    &= \epsilon_{i,j} \left(t\right) + \mathbb{1}\left(a_{t+1} = i,j \right) + t \bar{\alpha}_{i,j} \left(t\right) - \left(t+1\right) \bar{\alpha}_{i,j} \left(t+1\right) \label{le1eq3} \\
    &= \epsilon_{i,j} \left(t\right) + \mathbb{1}\left(a_{t+1} = i,j \right) -\alpha_{i,j}\left(t+1\right) \label{le1eq4} \\
    &\leq \epsilon_{i,j} \left(t\right) + \mathbb{1}\left(a_{t+1} = i,j \right) \label{le1eq5}
\end{align}
Next, we show that there exists $t_0" = t_0"\left(\epsilon\right)$ such that for all $t\geq t_0"$ we have $\left\{ a_{t+1} = i,j \right\} \subset \left\{ \epsilon_{i,j}\left(t\right) \leq 9t\epsilon \right\}$. We have from sampling rule $\left\{ a_{t+1} = i,j \right\} \subset \chi_1\left(t\right) \cup  \chi_2\left(t\right)$ where
\begin{align}
    \chi_1\left(t\right) &= \left\{ (i,j) = \argmin_{m,n \in \mathcal{L}} N_{m,n}\left(t\right) - \sum_{s=1}^t \alpha^*_{m,n}\left(s\right) \right\} \label{le2eq1} \\
    \chi_2\left(t\right) &= \left\{ (i,j) = \argmin_{m,n \in \mathcal{L}} N_{m,n}\left(t\right) < \sqrt{t}\right\} \label{le2eq2}
\end{align}
Let us suppose $\chi_1\left(t\right)$ holds true, then for all $t \geq t_0'$, we have
\begin{align}
    \epsilon_{i,j} \left(t\right) &= N_{i,j}\left(t\right) - t \bar{\alpha}_{i,j} \left(t\right) \label{le3eq1} \\
    &\overset{(\ref{le2eq1})}{=} \min_{m,n \in \mathcal{L}} N_{m,n}\left(t\right) - \sum_{s=1}^t \alpha^*_{m,n}\left(s\right) \label{le3eq2} \\
    &\leq 0 \leq 9t\epsilon\label{le3eq3}
\end{align}
Now, suppose that $\chi_2 \left(t\right)$ holds true for $t>\left(\dfrac{1}{\epsilon}\right)^2$, then we have
\begin{align}
    \epsilon_{i,j} \left(t\right) &= N_{i,j}\left(t\right) - t \bar{\alpha}_{i,j} \left(t\right) \label{le12eq1} \\
    &\overset{(\ref{le2eq2})}{\leq} \sqrt{t} - t \bar{\alpha}_{i,j} \left(t\right) \label{le12eq2} \\
    &\leq \dfrac{t}{\sqrt{t}} \label{le12eq3} \\
    &\leq 9t \epsilon \label{le12eq7} 
\end{align}
Hence, we have $\epsilon_{i,j}\left(t+1\right)$ being bounded by
\begin{align}
     \epsilon_{i,j} \left(t+1\right) &\leq \epsilon_{i,j} \left(t\right) + \mathbb{1}\left(\epsilon_{i,j} \left(t\right) \leq 9t \epsilon \right) \label{le4eq1}
\end{align}
We now prove by induction that $\epsilon_{i,j} \left(t\right) \leq \max\left\{\epsilon_{i,j}\left(t_0"\right) , 9t \epsilon + 1 \right\}$. We clearly see that it holds for $t=t_0"$. Now if $\epsilon_{i,j} \left(t\right) \leq 9t\epsilon$, we have
\begin{align}
     \epsilon_{i,j} \left(t+1\right) &\leq \epsilon_{i,j} \left(t\right) + \mathbb{1}\left(\epsilon_{i,j} \left(t\right) \leq 9t\epsilon \right) \label{le5eq1} \\
     &\leq 9t\epsilon + 1  \label{le5eq2} \\
     &\leq \max\left\{\epsilon_{i,j}\left(t_0"\right) , 9t \epsilon + 1 \right\} \label{le5eq3} \\
     &\leq \max\left\{\epsilon_{i,j}\left(t_0"\right) , 9\left(t+1\right)\epsilon + 1 \right\} \label{le5eq4} \; \forall i,j \in \mathcal{L}
\end{align}
whereas if $\epsilon_{i,j} \left(t\right) > 9t\epsilon$, then
\begin{align}
    \epsilon_{i,j} \left(t+1\right) &\leq \epsilon_{i,j} \left(t\right) \label{le6eq1} \\
    &\leq \max\left\{\epsilon_{i,j}\left(t_0"\right) , 9t \epsilon + 1 \right\}  \label{le6eq2} \\
    &\leq \max\left\{\epsilon_{i,j}\left(t_0"\right) , 9\left(t+1\right)\epsilon + 1 \right\} \label{le6eq3} \; \forall i,j \in \mathcal{L}
\end{align}
Because $\sum_{(m,n) \in \mathcal{L}} \epsilon_{m,n} \left(t\right) = 0$, we have 
\begin{align}
    \epsilon_{i,j} \left(t\right) &= -\sum_{(i',j') \in (\mathcal{L}\times \mathcal{L}) \backslash (i,j)} \epsilon_{i',j'}\left(t\right) \label{le7eq1} \\
    &\geq -\left( ^LC_2 - 1 \right) \max_{(i',j') \in (\mathcal{L}\times \mathcal{L}) \backslash (i,j)} \max\left\{\epsilon_{i',j'}\left(t_0"\right) , 9t\epsilon + 1 \right\} \label{le7eq2}
\end{align}
for all $i,j \in \mathcal{L}$. Thus, it follows that 
\begin{align}
    |\epsilon_{i,j} \left(t\right)| &\leq \left( ^LC_2 - 1 \right) \max_{(i',j') \in (\mathcal{L}\times \mathcal{L}) \backslash (i,j)} \max\left\{\epsilon_{i',j'}\left(t_0"\right) , 9t\epsilon + 1 \right\} \label{le8eq1} \\
    &\leq \left( ^LC_2 - 1 \right) \max\left\{t_0", 9t\epsilon + 1\right\} \label{le8eq2} \\
    &= \left( ^LC_2 - 1 \right) t \max\left\{\frac{t_0"}{t}, 9 \epsilon + \dfrac{1}{t} \right\} \label{le8eq3} \\
    &\leq 10 \left( ^LC_2 - 1 \right) t \epsilon \label{le8eq4}
\end{align}
for all $t \geq t_1 = \frac{1}{\epsilon}\max\left\{t_0", 10\right\}$, which in turn gives us
\begin{align}
    d_\infty\left( \left(N_{i,j}\left(t\right)/t \right)_{i,j \in \mathcal{L}}, S\right) &\leq d_\infty\left( \left(N_{i,j}\left(t\right)/t\right)_{i,j \in \mathcal{L}}, \hat{\alpha}\left(t\right)\right) \label{le11eq1} \\
    &\leq d_\infty\left(\left(N_{i,j}\left(t\right)/t \right)_{i,j \in \mathcal{L}}, \bar{\alpha}\left(t\right)\right) + d_\infty\left(\bar{\alpha}\left(t\right), \hat{\alpha}\left(t\right)\right) \label{le11eq2} \\
    &\leq \max_{i,j \in \mathcal{L}} \left|\dfrac{N_{i,j}\left(t\right)}{t} - \bar{\alpha}_{i,j}\left(t\right) \right| + 9\epsilon \label{le11eq3} \\
    &= \max_{i,j \in \mathcal{L}} \dfrac{\left|\epsilon_{i,j}\left(t\right)\right|}{t} + 9\epsilon \label{le11eq4} \\
    &\leq 10 \epsilon \left( ^LC_2 - 1 \right) + 9\epsilon\label{le11eq5}
\end{align}

\begin{lemma}
\label{lemma: lambert}
    For any two constants $k_1 > 0$, $k_2 > 0$ and for every $\gamma \geq 1$, from \cite{garivier2016optimal} we have
    \begin{align}
        \inf\left\{t \geq 1: tk_1 \geq \log\left(k_2t^\alpha\right)\right\} \leq \dfrac{\gamma}{k_1}\left(\log\dfrac{k_2e}{k_1^\alpha} + \log\log\dfrac{k_2}{k_1^\alpha}\right) \label{la1eq1}
    \end{align}
\end{lemma}

\begin{lemma}
\label{lemma: C}
    Given $C\left(x\right)$ as defined in Definition \ref{def: C_exp}, as $\delta \rightarrow 0$ we have $C\left(\dfrac{\log\left(\frac{L-1}{\delta}\right)}{L-1}\right)$ bounded by
    \begin{align}
        C\left(\dfrac{\log\left(\frac{L-1}{\delta}\right)}{L-1}\right) \leq \left(1+\upsilon\right)\left(\dfrac{\log\left(\frac{L-1}{\delta}\right)}{L-1} + 4\log\left( 1 + \dfrac{\log\left(\frac{L-1}{\delta}\right)}{L-1} + \sqrt{\dfrac{2\log\left(\frac{L-1}{\delta}\right)}{L-1}} \right)\right)
    \end{align}
    where $\upsilon \rightarrow 0$, as $x \rightarrow \infty$
\end{lemma}
\textbf{Proof of Lemma \ref{lemma: C}:}
Recall that 
\begin{align}
        C\left(x\right) &= 2\tilde{h}_{3/2}\left(\dfrac{h^{-1}\left(1+x\right) + \log\left(\pi^2/3 \right)}{2}\right) \label{sc5eq1} \\
        &\leq 2\tilde{h}_{3/2}\left(\dfrac{1 + x + \log\left(1 + x + \sqrt{2x}\right) + \log\left(\pi^2/3 \right)}{2}\right) \label{sc5eq2} \\
        &\leq 2\tilde{h}_{3/2}\left(\dfrac{x + 2\log\left(1 + x + \sqrt{2x}\right) }{2}\right) \label{sc5eq3} 
\end{align}
where the final inequality, holds for all $x$ such that $\log\left(1 + x + \sqrt{2x}\right) > \log\left(\pi^2/3 \right) + 1$. Now, let
\begin{align}
    h^{-1}\left(\dfrac{x + 2\log\left(1 + x + \sqrt{2x}\right) }{2}\right) &\leq  \resizebox{0.8\columnwidth}{!}{$\dfrac{x + 2\log\left(1 + x + \sqrt{2x}\right)}{2} + \log\left( \dfrac{x + 2\log\left(1 + x + \sqrt{2x}\right) }{2} + \sqrt{\left(x + 2\log\left(1 + x + \sqrt{2x}\right)-2 \right)}\right)$} \label{sc6eq2}\\
    &\leq \dfrac{x + 2\log\left(1 + x + \sqrt{2x}\right)}{2} + \log\left(1 + x + \sqrt{2x}\right) \label{sc6eq3}\\
    &= \dfrac{x + 4\log\left(1 + x + \sqrt{2x}\right)}{2} \label{sc6eq4}
\end{align}
where \eqref{sc6eq3} holds true for all $x > k_1$, such that $k_1 \in \mathbb{N}^+$. Now from the definition of $\tilde{h}_z\left(y\right)$, for every $y>h\left(\log\left(1/z\right)\right)$ we have $\tilde{h}_z\left(y\right) = e^{1/h^{-1}\left(y\right)}h^{-1}\left(y\right)$. Therefore, there exists some $k_2 \in \mathbb{N}^+$ such that for all $x>k_2$, we have
\begin{align}
    C\left(x\right) &\leq 2\tilde{h}_{3/2}\left(\dfrac{x + 2\log\left(1 + x + \sqrt{2x}\right) }{2}\right) \label{sc12eq1} \\
    &\leq 2\left(e^{\frac{2}{x + 4\log\left(1 + x + \sqrt{2x}\right)}} \left(\dfrac{x + 4\log\left(1 + x + \sqrt{2x}\right) }{2}\right)\right) \label{sc12eq2} \\
    &\leq \left(1+\upsilon\right)\left(x + 4\log\left( 1 + x + \sqrt{2x} \right)\right) \label{sc12eq3}
\end{align}
where $\upsilon \rightarrow 0 $ as $x \rightarrow \infty$ and \eqref{sc12eq2} holds true for all $x>k_3$, where $k_3 \in \mathbb{N}^+$. Now, let $x = \frac{\log\left(\frac{L-1}{\delta}\right)}{L-1}$ and $k = \max\{k_1, k_2, k_3\}$, then we know that as $\delta \rightarrow 0$, $x$ is guaranteed to be greater than $k$. Therefore, on substituting the value of $x$ in \eqref{sc12eq3}, we have the desired result.

\textbf{Proof of Theorem \ref{theorem: sample complexity}:}
Consider the event 
\begin{align}
    \chi = \left\{d_\infty\left(\left( N_{i,j}\left(t\right)/t \right)_{i,j \in \mathcal{L}}, \alpha^*\left(\nu\right)\right)\xrightarrow{t \rightarrow \infty} 0, \hat{\nu}\left(t \right) \xrightarrow{t \rightarrow \infty} \nu \right\} \label{sc1eq1}
\end{align}
From Lemma \ref{lemma: tracking}, we have $\chi$ occur with probability $1$ under the DCTAS algorithm. Now from the continuity of $\phi$, we know that there exists an open neighborhood of $\left\{ \nu \right\} \times \alpha^*\left(\nu\right)$, say $U=U\left( \epsilon \right)$ such that
\begin{align}
    \phi\left( \nu_0, \alpha_0\right) &\geq \left(1+\epsilon\right)^{-1}\phi\left(\nu, \alpha^*\right) \label{sc2eq1} \\
    &= \left(1+\epsilon\right)^{-1} \min_{i \neq 1} \left( \sum_{j \in \mathcal{L} \backslash i} \dfrac{\alpha_{i,j}}{\sum_{(m,n) \in \mathcal{K}} \alpha_{m,n} (c_m+c_n)} d\left(p_{i,j}, \max{(0.5, p_{i,j})}\right) \right) \label{sc2eq2} \\
    &= \left(1+\epsilon\right)^{-1} \min_{i \neq 1} \left( \sum_{j \in \mathcal{L} \backslash i} \dfrac{w_{i,j}}{c_i + c_j} d\left(p_{i,j}, \max{(0.5, p_{i,j})}\right)\right) \label{sc2eq3} \\
    &= \left(1+\epsilon\right)^{-1}c^*\left(\nu\right)^{-1} \label{sc2eq4} \; \forall\left(\nu_0, w_0\right) \in U
\end{align}
Next, under the event $\chi$, there exists $n_0 = n_0\left(\epsilon\right)$ such that $\left( \hat{\nu}\left(t\right), \left(N_{i,j}\left(t\right)/t\right)_{i,j \in \mathcal{L}} \right) \in U$ for all $t \geq n_0$, and consequently
\begin{align}
    \phi\left( \hat{\nu}\left(t\right), \left(N_{i,j}\left(t\right)/t\right)_{i,j \in \mathcal{L}} \right) &\geq \left(1+\epsilon\right)^{-1}c^*\left(\nu\right)^{-1} \label{sc3eq1} \; \forall t \geq n_0
\end{align}
Because $\hat{\nu}\left(t \right) \xrightarrow{t \rightarrow \infty} \nu$ and we have a unique best arm, there exists $n_1$ such that for all $t\geq n_1$, the GLRT statistic can be written as
\begin{align}
    Z\left(t\right) &= \min_{j \neq 1} \left(\sum_{k \in \mathcal{L} \backslash j} N_{j,k}\left(t\right) d(\hat{p}_{j,k}\left(t\right), \max(\hat{p}_{j,k}\left(t\right), 0.5)) - \sum_{k \in \mathcal{L} \backslash 1} N_{1,k}\left(t\right) d\left(\hat{p}_{1,k}, \max\left(\hat{p}_{1,k}\left(t\right), 0.5\right)\right)\right) \label{sc4eq1} \\
    &= \min_{j \neq 1} \sum_{k \in \mathcal{L} \backslash j} N_{j,k}\left(t\right) d(\hat{p}_{j,k}\left(t\right), \max(\hat{p}_{j,k}\left(t\right), 0.5)) \label{sc4eq2} \\
    &= t \left[\min_{j \neq 1} \sum_{k \in \mathcal{L} \backslash j} \dfrac{N_{j,k}\left(t\right)}{t} d(\hat{p}_{j,k}\left(t\right), \max(\hat{p}_{j,k}\left(t\right), 0.5))\right] \label{sc4eq3} \\
    &= J\left(t\right) \left[\min_{j \neq 1} \sum_{k \in \mathcal{L} \backslash j} \dfrac{N_{j,k}\left(t\right)/t}{\sum_{(m,n) \in \mathcal{K}} N_{m,n}\left(t\right) \left(c_m+c_n\right)/t} d(\hat{p}_{j,k}\left(t\right), \max(\hat{p}_{j,k}\left(t\right), 0.5))\right] \label{sc4eq4}\\    
    &= J\left(t\right)\phi\left( \hat{\nu}\left(t\right), \left(N_{j,k}\left(t\right)/t\right)_{j,k \in \mathcal{L}} \right) \label{sc4eq5} \\
    &\overset{\eqref{sc3eq1}}{\geq} J\left(t\right)\left(1+\epsilon\right)^{-1}c^*\left(\nu\right)^{-1} \label{sc4eq6}
\end{align}
Next, let $\log\left(B\right) = 4\left(L-1\right)\log\left(1+\frac{\log\left(\frac{L-1}{\delta}\right)}{L-1}\right) + \sqrt{\frac{2\log\left(\frac{L-1}{\delta}\right)}{L-1}}$, than from the definition of $\beta\left(t, \delta\right)$ and Lemma \ref{lemma: C}, we have
\begin{align}
    \beta\left(t, \delta\right) &\leq 3(L-1)\log\left(1 + \log\left(\dfrac{t}{L-1}\right)\right) + \left(1+\upsilon\right)\left(\log\left(\frac{L-1}{\delta}\right) + \log\left(B\right)\right) \label{sc7eq1} \\
    &\leq \left(1+\upsilon\right)\left(3(L-1)\log\left(1 + \log\left(\dfrac{t}{L-1}\right)\right) + \log\left(\frac{L-1}{\delta}\right) + \log\left(B\right)\right) \label{sc7eq3} \\
    &\leq \left(1+\upsilon\right)\left(3(L-1)\log\left(\frac{t}{L-1}\right)^{\frac{1}{3(L-1)}} + \log\left(\frac{L-1}{\delta}\right) + \log\left(B\right)\right) \label{sc7eq2} \\
    &= \left(1+\upsilon\right)\log\left(\frac{Bt}{\delta}\right) \label{s8eq2} 
\end{align}
where \eqref{sc7eq2} holds true only for all $t>n_2$, such that $n_2 \in \mathbb{N}^+$. We also have
\begin{align}
    J\left(\tau_\delta\right) &= J\left(\inf\left\{t \geq \max\left\{n_0, n_1, n_2 \right\} \mid Z\left(t\right) \geq \beta\left(t, \delta \right) \right\}\right)  \label{sc9eq1} \\
    &\overset{(\ref{s8eq2})}{\leq} J\left(\inf\left\{t \geq \max\left\{n_0, n_1, n_2\right\} \mid  J\left(t\right)\left(1+\epsilon\right)^{-1} \left(1+\upsilon\right)^{-1}c^*\left(\nu\right)^{-1} \geq \log\left(\dfrac{Bt}{\delta}\right)\right\}\right) \label{sc9eq2} \\
    &\leq J\left(n_0\right) \cup J\left(n_1\right) J\left(n_2\right) \cup J\left(\inf\left\{t \mid J\left(t\right)\left(1+\epsilon\right)^{-1}\left(1+\upsilon\right)^{-1}c^*\left(\nu\right)^{-1} \geq \log\left(\dfrac{BJ\left(t\right)}{\min\left(\mathcal{C} \right)\delta}\right) \right\}\right) \label{sc9eq3}
\end{align}
Now from Lemma \ref{lemma: lambert}, we have
\begin{align}
    \resizebox{\columnwidth}{!}{$ J\left(\inf\left\{t \mid J\left(t\right)\left(1+\epsilon\right)^{-1}\left(1+\upsilon\right)^{-1}c^*\left(\nu\right)^{-1} \geq \log\left(\dfrac{BJ\left(t\right)}{\min\left(\mathcal{C} \right)\delta}\right) \right\}\right) \leq \left(1+\epsilon\right)\left(1+\upsilon\right)c^*\left(\nu\right)\left(\log\left(\dfrac{Be\left(\left(1+\epsilon\right)\left(1+\upsilon\right)c^*\left(\nu\right)\right)}{\min\left(\mathcal{C} \right)\delta}\right) + \log \log\left(\dfrac{B\left(\left(1+\epsilon\right)\left(1+\upsilon\right)c^*\left(\nu\right)\right)}{\min\left(\mathcal{C} \right)\delta}\right)\right) + \mathcal{O}\left(\max\left(\mathcal{C}\right)\right) $} \label{sc10eq1}
\end{align}
Therefore from \eqref{sc9eq3} and \eqref{sc10eq1} for every $\delta \in (0,1)$ on letting $\epsilon$ and $\upsilon$ tending to $0$, we have
\begin{align}
    \limsup_{\delta \rightarrow 0} \dfrac{J\left(\tau_{\delta}\right)}{\log\left(1/\delta\right)} &\leq c^*\left(\nu\right) \label{sc11eq1} 
\end{align}
